# Supplementary material for: VECHR: A Dataset for Explainable and Robust Classification of Vulnerability Type in the European Court of Human Rights
Source: arXiv:2310.11368 source file (2023-10-24)
Supplement: Supplementary file 1 [file appendix_dataset.tex]

\begin{figure}[h!]
    \centering
    \includegraphics[width=8cm]{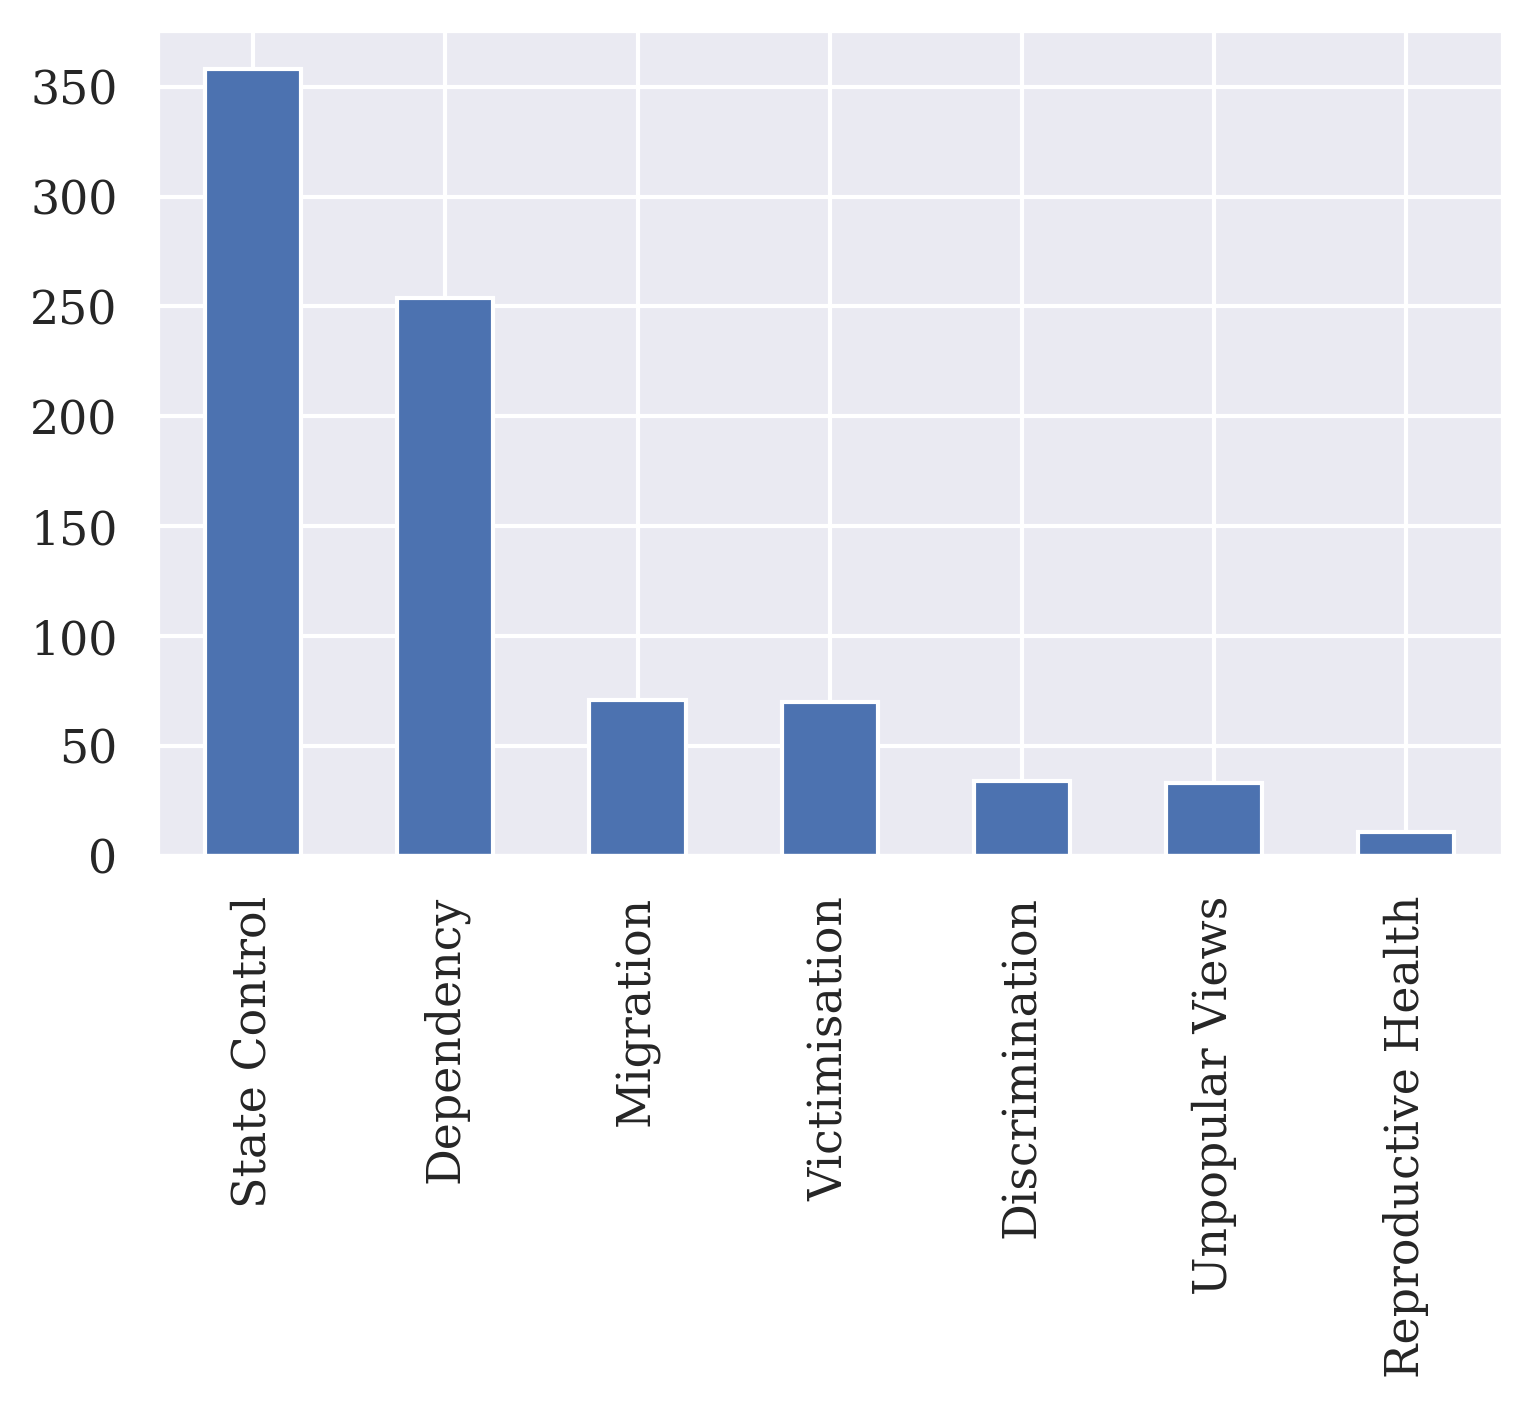}
    \caption{Frequency of vulnerability type annotations.}
    \label{fig:label-count}
\end{figure}

\begin{figure}[h!]
    \centering
    \includegraphics[width=8cm]{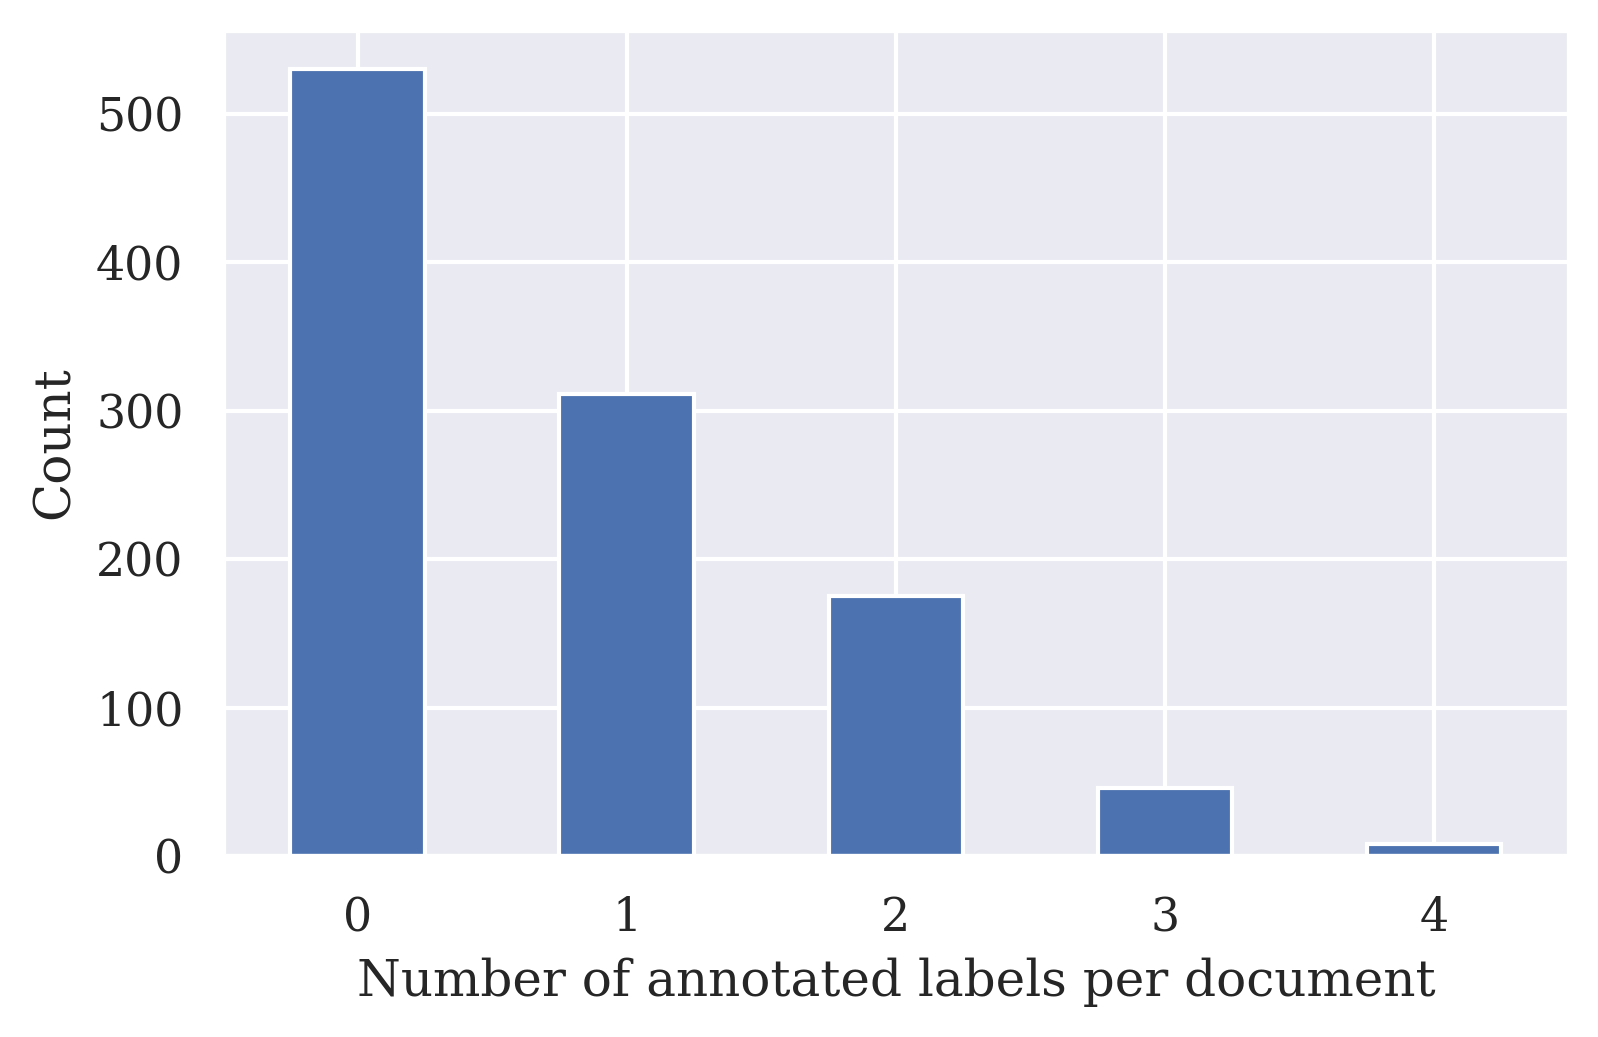}
    \caption{Distribution of number of annotated labels per document.}
    \label{fig:multi-count}
\end{figure}

\begin{figure}[h!]
    \centering
    \includegraphics[width=8cm]{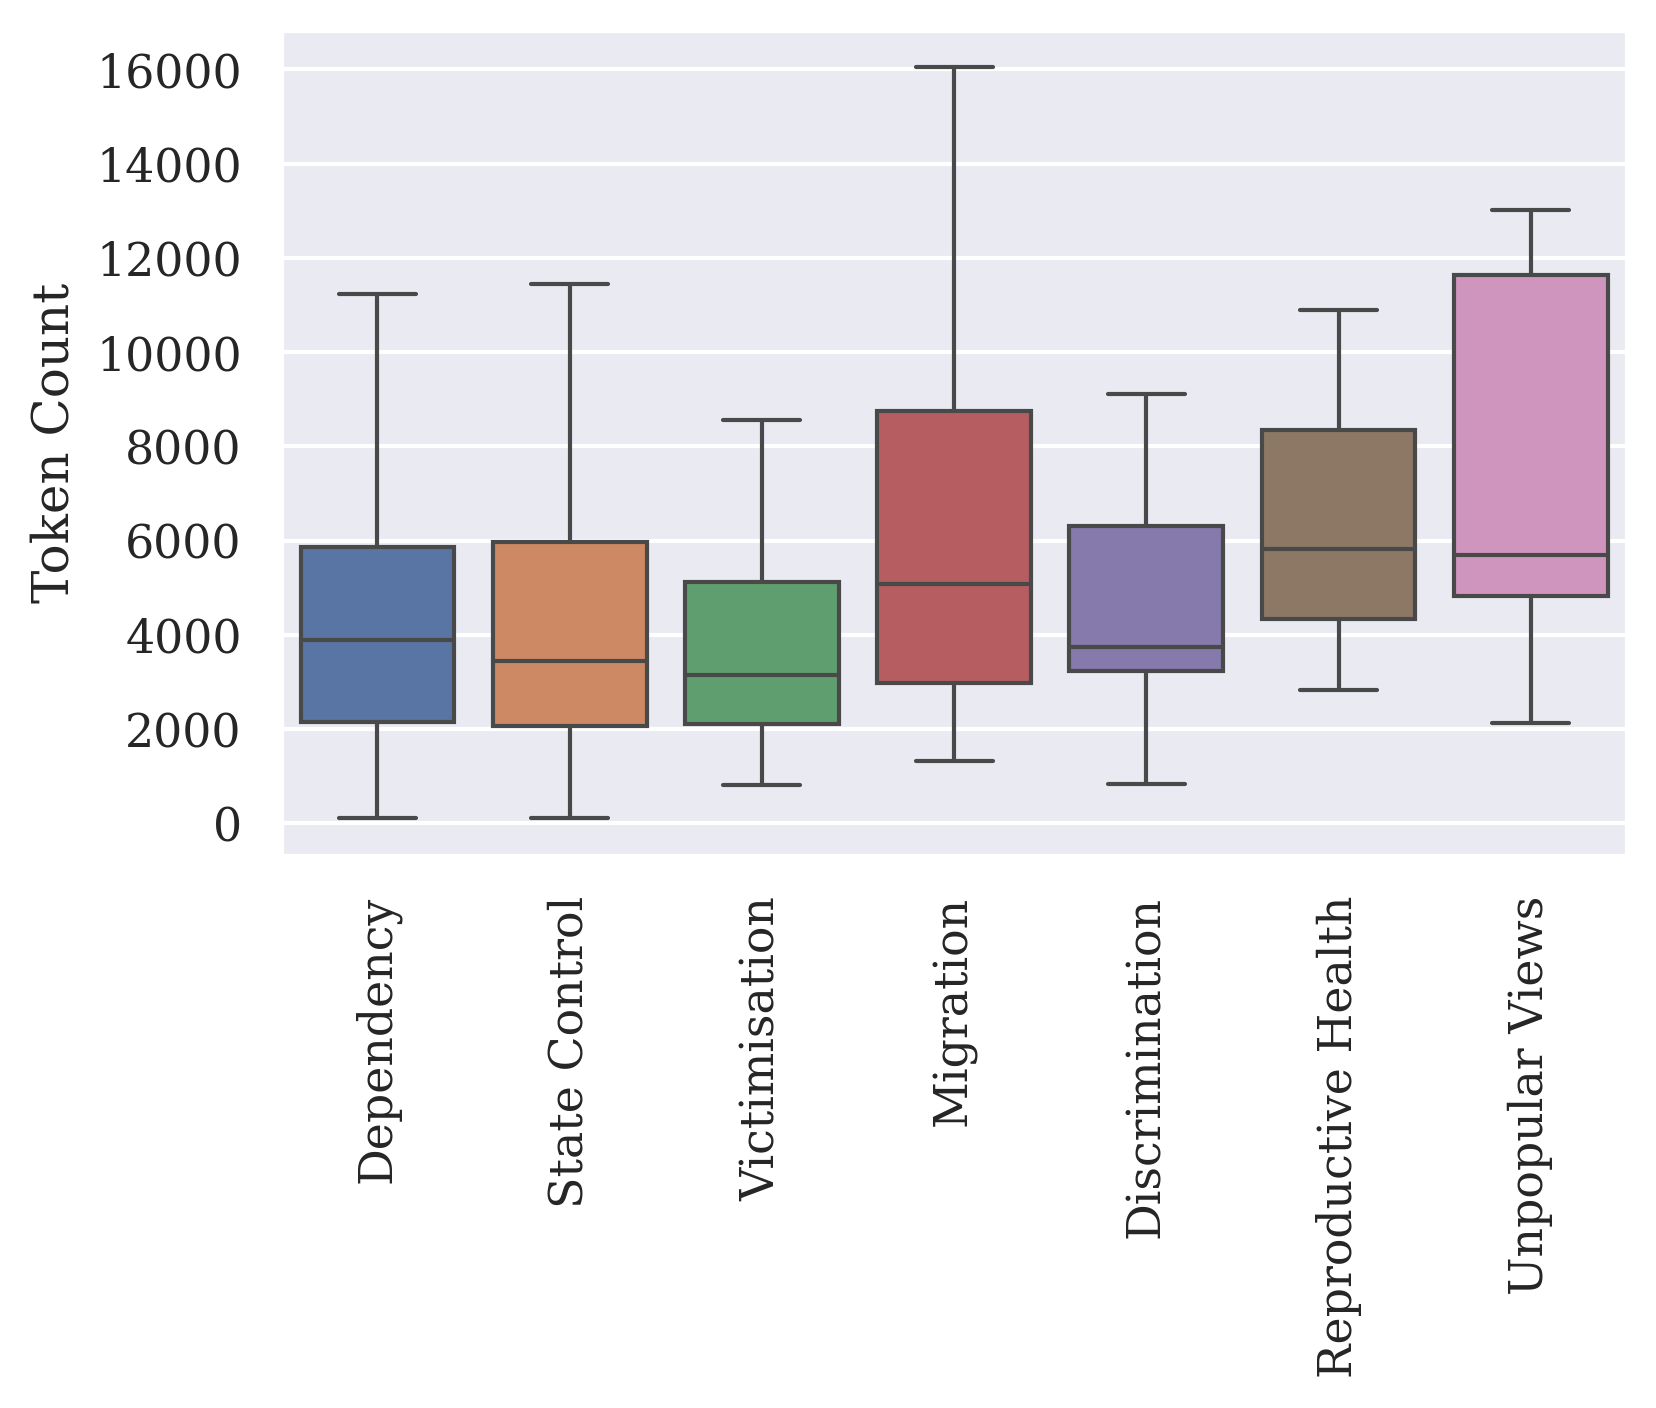}
    \caption{Box plot of the token count per typology.}
    \label{fig:boxplot-token-count}
\end{figure}

\begin{figure}[h!]
    \centering
    \includegraphics[width=8cm]{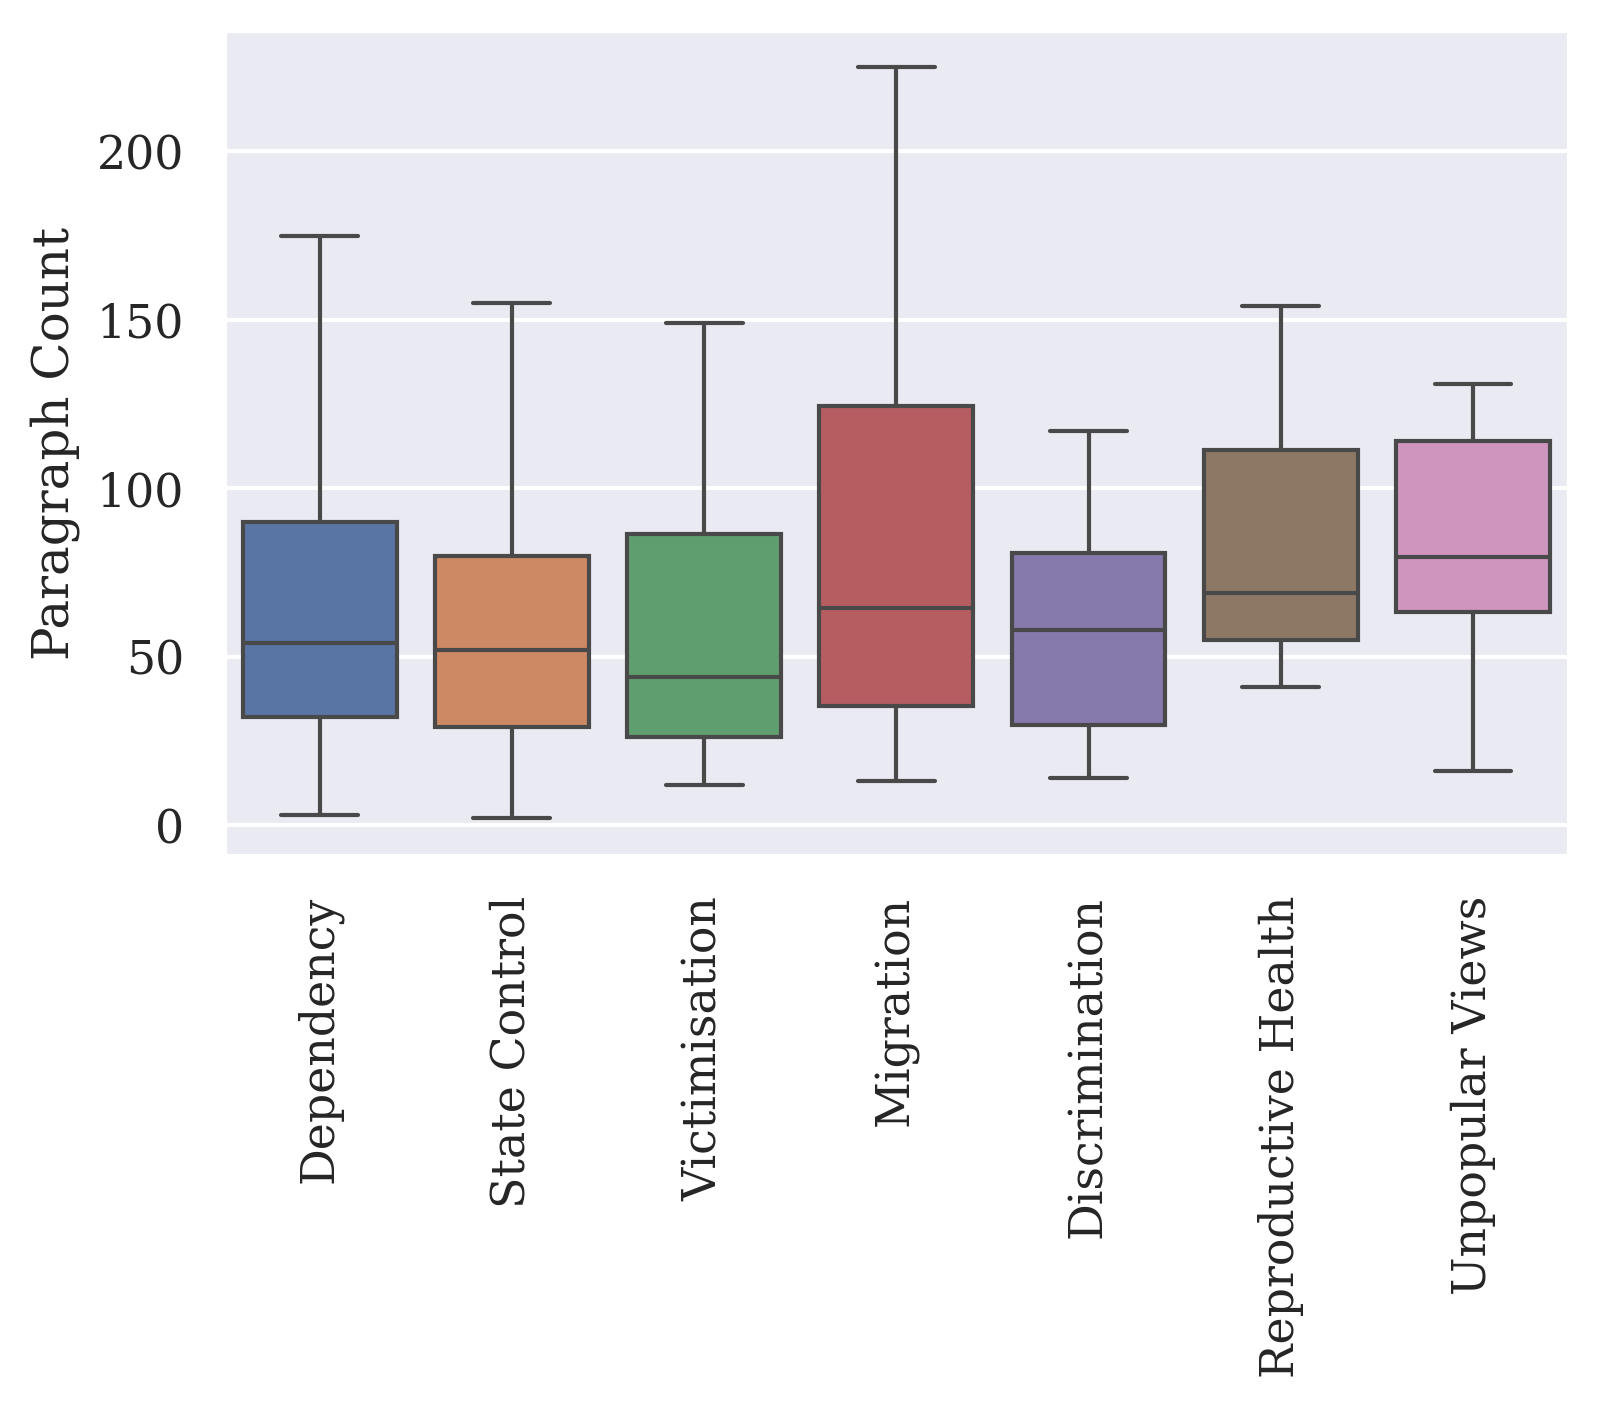}
    \caption{Box plot of the number of paragraphs per typology.}
    \label{fig:boxplot-seg-count}
\end{figure}

\begin{figure}[h!]
    \centering
    \includegraphics[width=8cm]{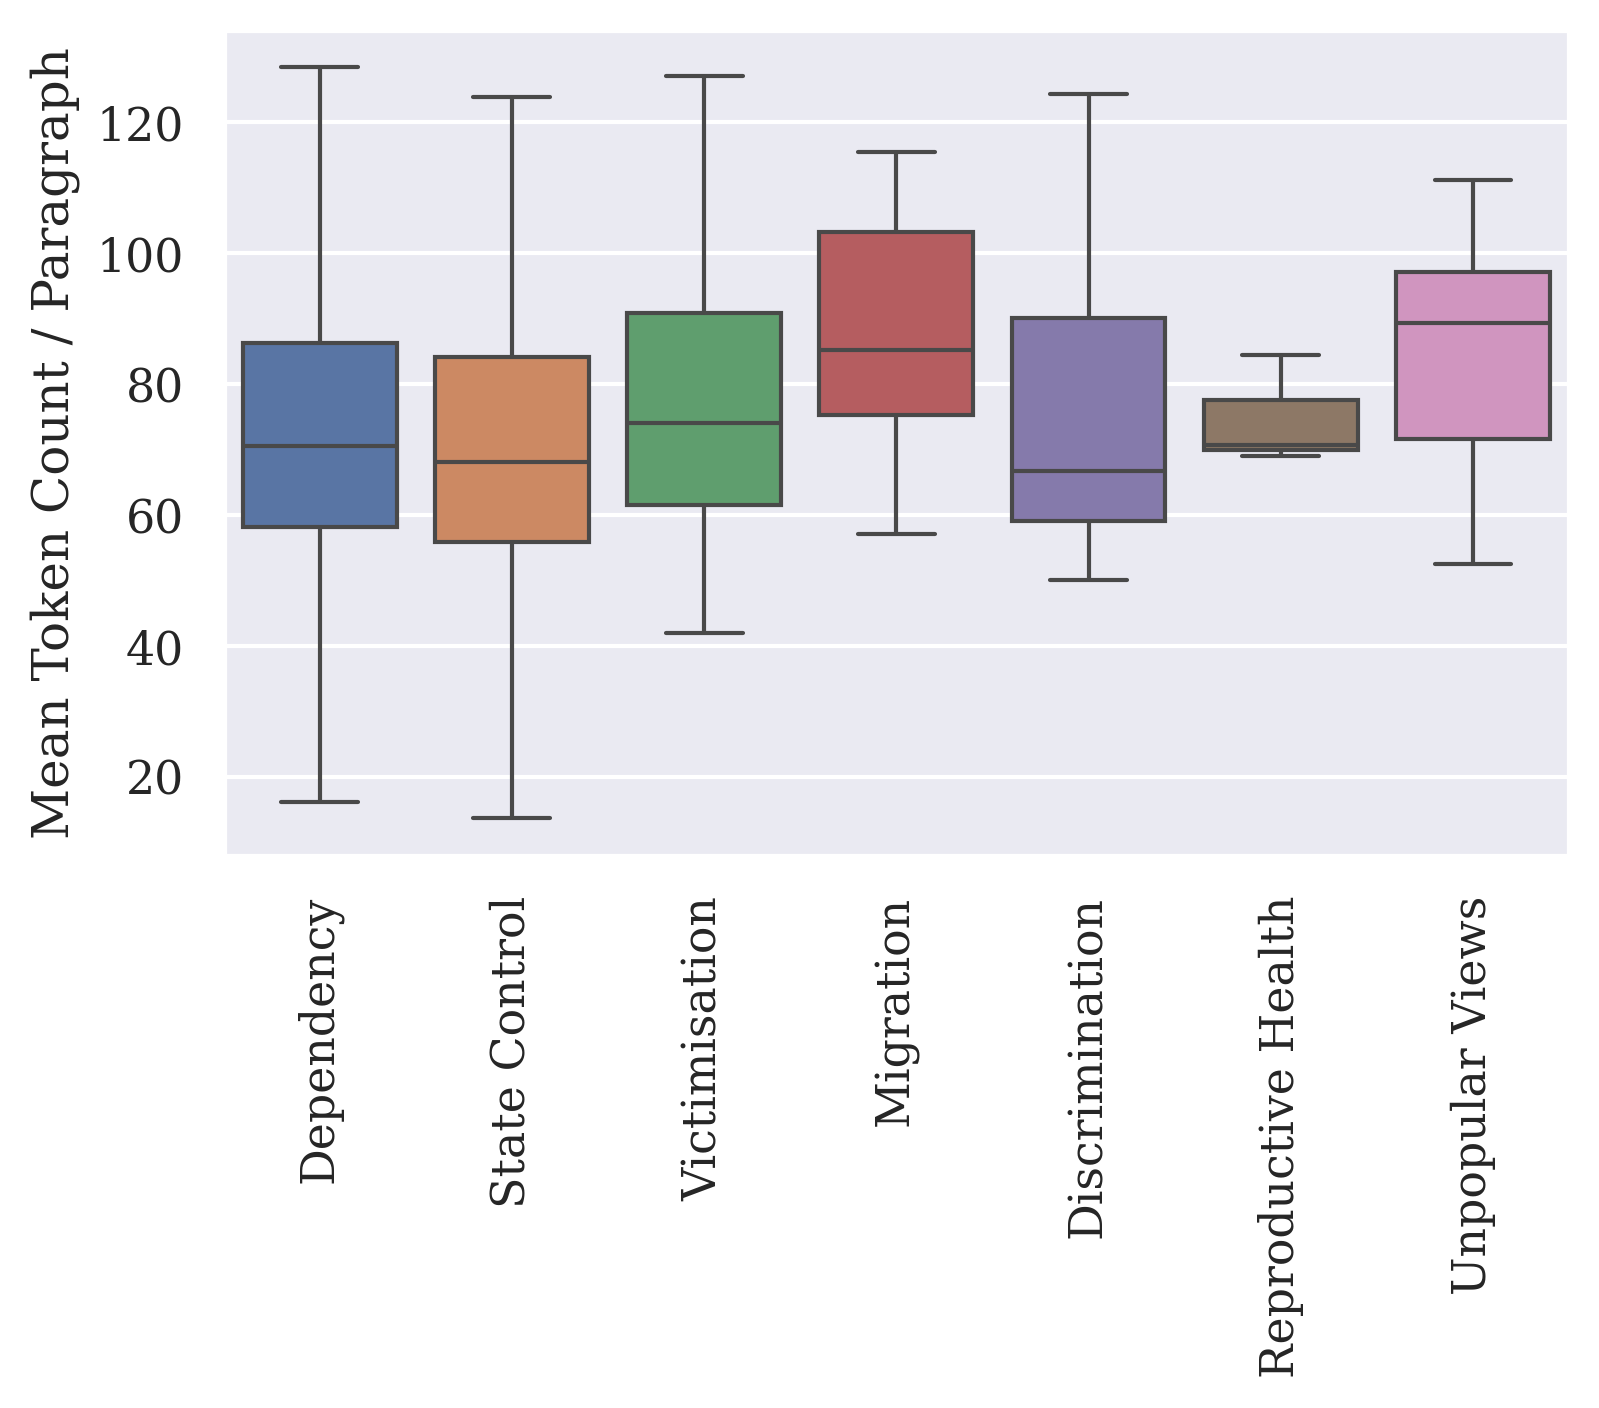}
    \caption{Box plot of the mean number of tokens per paragraph per typology.}
    \label{fig:boxplot-token-seg}
\end{figure}
